# Supplementary material for: Dilemma First Search for Effortless Optimization of NP-Hard Problems
Source: arXiv:1609.03545 source file (2016-09-12)
Supplement: Supplementary file 1 [file paper_dilemma_tree_search_appendix.tex]

\begin{appendix}
 \section{Appendix: Proofs}

 \subsection{Theorem~\ref{theo:greedy} [Base case]}
When the tree is unexplored, the greedy solution finds $\operatorname*{arg\,max}_{\hat{S}} P_{\opt}(\hat{S})$ when exploring at most depth $d$ nodes.

% PROOOOOF
\begin{proof}
 When exploring at most d nodes, only one solution candidate can be built.
 We have $P_{\best}(A_k|S_k) \ge P_{\best}(A_j \ne A_k|S_k)$ and $P_{\best}(A_k|S_k) \ge P_{\uni}$ (from As.~\ref{ass:proba}).
 If a candidate solution contains $P_{\best}(A_k|S_k)$, its expected probability is always higher than any other unexplored candidate solution whose expected probability is uniform (from Eq.~\eqref{eq:popt} and Lemma~\ref{lem:bounderies}).
 %By induction, in the initial state the candidate solution with the highest expected probability is the one containing $arg_Amax P_{\best}(A_{i,0}|S_0)$, where $S_0$ is the root node.
%multiplying keeps the same order
\end{proof}

\subsection{Theorem~\ref{theo:next} [Inductive step]}
%Any not fully explored candidate solution is bounded by a longer not fully explored candidate solution if 
Given the set of $n^{th}$ most likely candidate solutions have been explored, the $(n+1)^{th}$ most likely candidate solution can be inferred by exploring at most d more nodes.

\begin{proof} [Proof sketch]
%Let $\mathcal{\hat{S}}_{unexp}$ be the set of unexplored candidate solutions.
The $n^{th}$ solution has a probability to yield the optimal solution $P_{\opt}(\hat{S}_{n})$ larger than any other unexplored candidate solutions $P_{\opt}(\hat{S})$, $\hat{S} \in \mathcal{\hat{S}}_{unexp}$.
Hence, finding the $P_{\opt}(\hat{S}_{n+1})$ is equivalent to finding:

\begin{equation} \label{eq:mindiff}
 \operatorname*{arg\,min}_{\alpha} (L_{\opt}(\hat{S_{n}}) - L_{\alpha})
\end{equation}
where $L(x) = log(P(x))$ is the positive log probability and $\alpha$ indicates the dilemmatic state $S_\alpha$ to change.
Thus, following Eq.~\eqref{eq:candidateProba} the current candidate solution is associated with the log probability:

\begin{equation} \label{eq:palpha}
 L_{\opt}(\hat{S_{n}}) = \sum_{k=1}^{d} L_{\best}(S_k)
\end{equation}

where $L_{\best}(S_k)$ is the highest log probability. Further, following Eq.~\eqref{eq:popt} + \eqref{eq:mindiff}, we have:
\begin{equation} \label{eq:lalpha}
 L_{\alpha} = \sum_{k=1}^{\depth(\alpha) - 1} L_{\best}(S_k) + L_{\best}'(S_{\alpha}) + \sum_{k=\depth(\alpha) + 1}^{d} L_{\uni}
\end{equation}
where $L_{\best}'(S_\alpha)$ is the highest log probability associated with an unexplored child state at $S_\alpha$.
%Hence, Eq.~\eqref{eq:mindiff} derived from Eq.~\eqref{eq:lalpha} + \eqref{eq:palpha} as:
Hence, replacing Eq.~\eqref{eq:lalpha} + \eqref{eq:palpha} in Eq.~\eqref{eq:mindiff} gives:

\begin{equation} \label{eq:lopt-lalpha}
%   \begin{aligned} 
% L_{\opt}(\hat{S_{n}}) - L_{\alpha} = & (L_{\best}(S_{\alpha}) - L'_{\best}(S_\alpha))\\
% 			      + & \sum_{k=\depth(\alpha) + 1}^d (L_{\best}(S_k) - L_{\uni})
%   \end{aligned}
L_{\opt}(\hat{S_{n}}) - L_{\alpha} = (L_{\best}(S_{\alpha}) - L'_{\best}(S_\alpha))  +  \sum_{k=\depth(\alpha) + 1}^d (L_{\best}(S_k) - L_{\uni})
\end{equation}
where the first term corresponds to the difference of log probabilities at the dilemmatic state $S_\alpha$, while the second term is the expected gain in log probability over a uniform log probability distribution in the remaining tree.
Once the state $S_\alpha$ to be modified has been found, a $\hat{S}_{n+1}$ candidate solution is built by a greedy search in the subtree whose root is $S_\alpha$ (see Theorem~\ref{theo:greedy}).
\end{proof}

To simplify the computation, we can approximate $L_{\best}(S_k) - L_{\uni}$ by a positive constant: $L_{\uni}$ is constant and $L_{\best}(S_k)$ can be assumed to be constant on average.
As a result, Eq.~\eqref{eq:lopt-lalpha} can be approximated by

\begin{equation} \label{eq:lopt-lalphaapprox}
%\begin{aligned} 
%   L_{\opt}(\hat{S_{n}}) - L_{\alpha} \approx & L_{\best}(S_{\alpha}) - L'_{\best}(S_\alpha) \\
%                                       + & (d - \depth(\alpha)) \cdot const.
  L_{\opt}(\hat{S_{n}}) - L_{\alpha} \approx L_{\best}(S_{\alpha}) - L'_{\best}(S_\alpha) + (d - \depth(\alpha)) \cdot const.
%\end{aligned}
\end{equation}

Hence, minimizing Eq.~\eqref{eq:lopt-lalphaapprox} is equivalent to finding:
%\begin{equation} \label{eq:popt-palphaapprox}
% arg_{\alpha}min   \frac{P_{\best}(S_{\alpha})}{P'_{\best}(S_\alpha) \cdot \alpha}
%\end{equation}

\begin{equation} \label{eq:lopt-lalphaapprox2}
  \operatorname*{arg\,min}_{\alpha} ( L_{\best}(S_{\alpha}) - L'_{\best}(S_\alpha) - \depth(\alpha) \cdot const.)
  %L_{\opt}(\hat{S}) - L_{\alpha} \approx L_{\best}(S_{\alpha}) - L'_{\best}(S_\alpha) + D - \alpha \ + 1) \cdot C
\end{equation}

where $S_{\alpha}$ indicates the state in the tree where the next most likely candidate solution should be greedily grown from. %where in the tree the next most likely expected candidate solution should be expanded.
The first term favours exploring states where the difference between the best and the second best option is small,
while second term gives preference to exploring candidate solutions re-using a large part of the initial solution.

 \end{appendix}
